# Supplementary material for: Active shooter detection and robust tracking utilizing supplemental synthetic data
Source: arXiv:2309.03381 source file (2023-09-06)
Supplement: Supplementary file 1 [file supplementary_temp.pdf]

# Supplementary information for Active shooter detection and robust tracking utilizing supplemental synthetic data

Joshua R. Waite<sup>1</sup>, Jiale Feng<sup>2</sup>, Riley Tavassoli<sup>3</sup>, Laura Harris<sup>3</sup>, Sin Yong Tan<sup>1</sup>, Subhadeep Chakraborty<sup>3</sup>, and Soumik Sarkar<sup>1</sup>

<sup>1</sup>Department of Mechanical Engineering, Iowa State University, Ames, IA 50011, USA

<sup>2</sup>Department of Computer Science, Iowa State University, Ames, IA 50011, USA

<sup>3</sup>Department of Mechanical Engineering, University of Tennessee, Knoxville, TN 37996, USA

\*soumiks@iastate.edu

## Results for all data combinations and gun class

A total of 71 data combinations were explored when training YOLOv8n.

### Detection with YOLOv8

The detection results for the gun class can be seen in Table S1. The combination column denotes the type of data used to train that model. When multiple data types are in an ID, it represents the order in which the data was used to train. For example, *Masked\_textured\_Real\_L* was first trained with masked synthetic data, followed by textured synthetic data, and finished with a large amount of real data. The following columns, UE5, UE4 & UE5, UE5 Augmented, and UE4 & UE5 Augmented, denote when the synthetic data is from only UE5 or also includes UE4 data and whether the textured synthetic data is augmented with camera sensor effects.

**Table S1.** YOLOv8n training results for the gun class

| Combination            |           | UE5    |          |           | UE4 & UE5 |         |           | UE5 Augmented |         |           | UE4 & UE5 Augmented |         |  |
|------------------------|-----------|--------|----------|-----------|-----------|---------|-----------|---------------|---------|-----------|---------------------|---------|--|
| ID                     | precision | recall | mAP50    | precision | recall    | mAP50   | precision | recall        | mAP50   | precision | recall              | mAP50   |  |
| Masked_L               | 0.431     | 0.03   | 0.0292   | 0.261     | 0.06      | 0.0755  | -         | -             | -       | -         | -                   | -       |  |
| Masked_M               | 0.0452    | 0.03   | 0.0205   | 0.025     | 0.05      | 0.00747 | -         | -             | -       | -         | -                   | -       |  |
| Masked_S               | 0.0323    | 0.12   | 0.0192   | 0.179     | 0.23      | 0.103   | -         | -             | -       | -         | -                   | -       |  |
| Textured_L             | 0.000423  | 0.07   | 0.000231 | 0         | 0         | 0.00805 | 1         | 0             | 0.00362 | 0         | 0                   | 0.0085  |  |
| Textured_M             | 0.0114    | 0.02   | 0.0039   | 1         | 0         | 0.00285 | 0         | 0             | 0.0051  | 1         | 0                   | 0.00336 |  |
| Textured_S             | 0.000827  | 0.16   | 0.000482 | 0.17      | 0.09      | 0.0951  | 0.231     | 0.01          | 0.0271  | 0.161     | 0.05                | 0.0389  |  |
| Real_L                 | 0.388     | 0.22   | 0.255    | -         | -         | -       | -         | -             | -       | -         | -                   | -       |  |
| Real_M                 | 1         | 0      | 0.00165  | -         | -         | -       | -         | -             | -       | -         | -                   | -       |  |
| Real_S                 | 0.00226   | 0.34   | 0.00169  | -         | -         | -       | -         | -             | -       | -         | -                   | -       |  |
| Masked_Real_L          | 0.514     | 0.211  | 0.277    | 0.45      | 0.196     | 0.154   | -         | -             | -       | -         | -                   | -       |  |
| Masked_Real_M          | 0.591     | 0.22   | 0.255    | 0.325     | 0.22      | 0.19    | -         | -             | -       | -         | -                   | -       |  |
| Masked_Real_S          | 0.401     | 0.17   | 0.17     | 0.207     | 0.04      | 0.056   | -         | -             | -       | -         | -                   | -       |  |
| Textured_Real_L        | 0.5       | 0.22   | 0.243    | 0.306     | 0.344     | 0.212   | 0.4       | 0.27          | 0.272   | 0.483     | 0.39                | 0.342   |  |
| Textured_Real_M        | 0.5       | 0.13   | 0.214    | 0.453     | 0.31      | 0.229   | 0.383     | 0.26          | 0.256   | 0.342     | 0.17                | 0.174   |  |
| Textured_Real_S        | 0.316     | 0.138  | 0.136    | 0.493     | 0.22      | 0.241   | 1         | 0             | 0.0179  | 0.449     | 0.22                | 0.189   |  |
| Masked_Textured        | 0         | 0      | 0.00329  | 0.674     | 0.07      | 0.0933  | 0.126     | 0.07          | 0.0427  | 0.0793    | 0.08                | 0.022   |  |
| Masked_Textured_Real_L | 0.0312    | 0.15   | 0.0144   | 0.442     | 0.21      | 0.232   | 0.425     | 0.21          | 0.227   | 0.205     | 0.18                | 0.0867  |  |
| Masked_Textured_Real_M | 0.608     | 0.16   | 0.18     | 0.346     | 0.21      | 0.183   | 0.445     | 0.28          | 0.313   | 0.652     | 0.2                 | 0.331   |  |
| Masked_Textured_Real_S | 0.847     | 0.18   | 0.26     | 0.592     | 0.189     | 0.231   | 0.548     | 0.22          | 0.227   | 0.418     | 0.23                | 0.195   |  |
| Textured_Masked        | 0.0699    | 0.01   | 0.0207   | 0.00901   | 0.03      | 0.0048  | 0.0778    | 0.02          | 0.0113  | 0.0224    | 0.03                | 0.0208  |  |
| Textured_Masked_Real_L | 0.456     | 0.2    | 0.239    | 0.227     | 0.16      | 0.152   | 0.459     | 0.21          | 0.247   | 0.335     | 0.23                | 0.236   |  |
| Textured_Masked_Real_M | 0.123     | 0.04   | 0.032    | 0.334     | 0.14      | 0.158   | 0.716     | 0.17          | 0.315   | 0.605     | 0.28                | 0.328   |  |
| Textured_Masked_Real_S | 0.317     | 0.02   | 0.0217   | 0.382     | 0.08      | 0.0723  | 0.479     | 0.23          | 0.213   | 0.278     | 0.12                | 0.071   |  |

Precision-recall curves for the shooter and gun classes combined for the different data types can be seen in Fig. S1. The lower gun detection performance brings down the overall performance, but the general trend of combined augmented data performing best is still prevalent.

### Tracking with Deep OC-SORT and OSNet ReID

Tracking PR curve results for all the data combinations can be seen in Fig. S2. While adding gun-based shooter confirmation generally improves performance, it seems limited to models already performing reasonably well. The models with lower initial

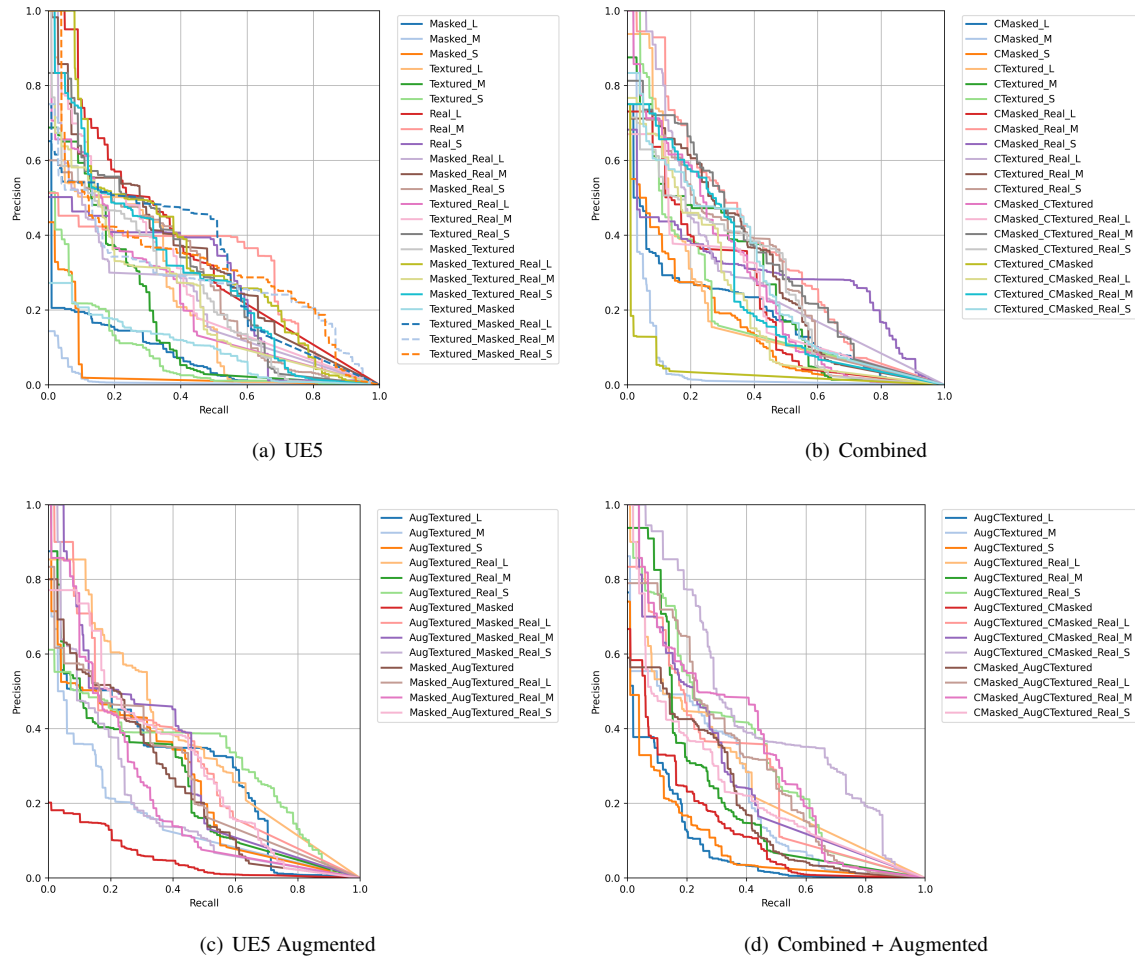

**Figure S1.** The testing results (PR curves) of different YOLOv8n models trained on different data combinations for the gun and shooter classes.

performance likely do not have sufficient quality gun detections to allow shooters to be properly assigned IDs.

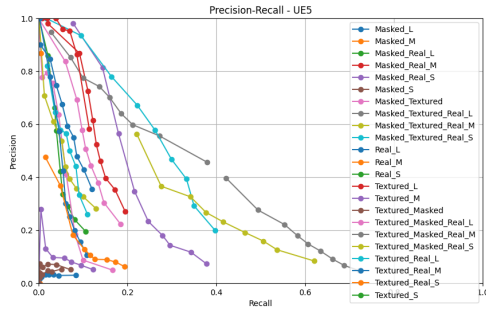

(a) Shooter Only

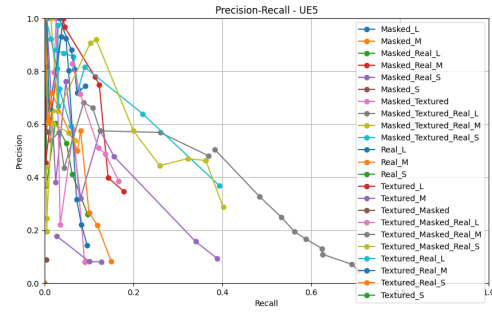

(b) Shooter Confirmed with Gun

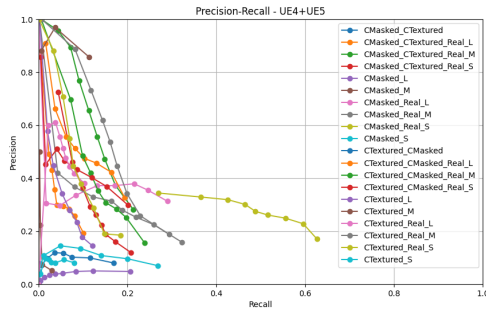

(c) Shooter Only

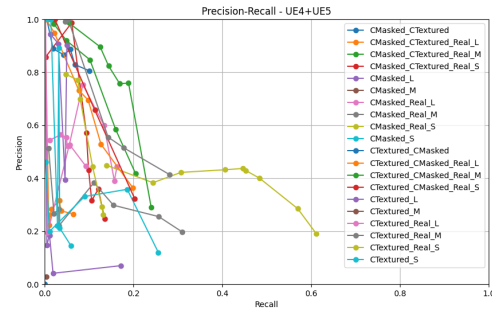

(d) Shooter Confirmed with Gun

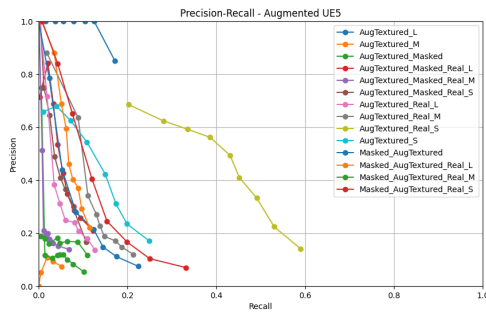

(e) Shooter Only

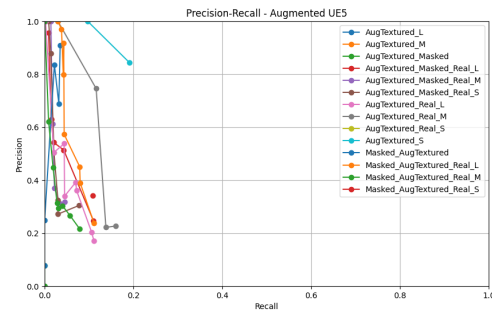

(f) Shooter Confirmed with Gun

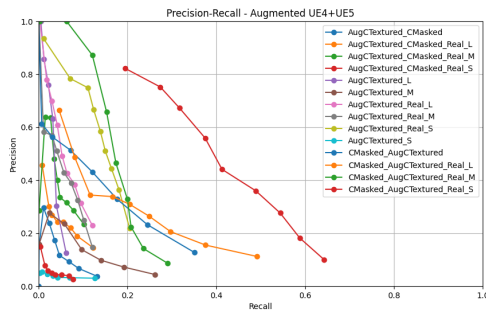

(g) Shooter Only

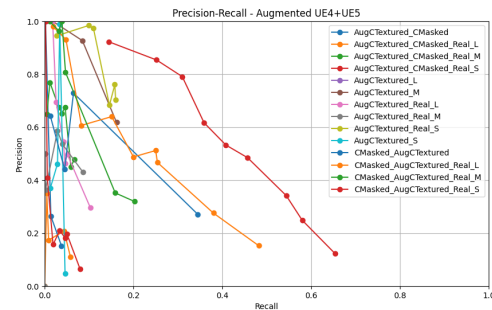

(h) Shooter Confirmed with Gun

**Figure S2.** The testing results (PR curves) for (a) tracking with only shooter detections and (b) tracking with shooter detections confirmed with a gun detection. Confidence thresholds for the gun and shooter detections were varied individually from 0.1 to 0.9.
